# Supplementary material for: Controlled gel expansion through colloid oscillation
Source: arXiv:2207.13605 source file (2022-07-27)
Supplement: Supplementary file 1 [file SM_sphere.pdf]

# Supplementary Material: Controlled network expansion through colloid oscillation

Guido L. A. Kusters,[1,*] Cornelis Storm,[1,2] and Paul van der Schoot[1]

[1]*Department of Applied Physics, Eindhoven University of Technology, The Netherlands*

[2]*Institute for Complex Molecular Systems, Eindhoven University of Technology, The Netherlands*

[*] g.l.a.kusters@tue.nl

## I. SELECTIVE FRICTION

In writing the dynamical equations (1)-(6) in the main text we assume that the polymer network does not screen the viscous friction of the colloid with the background fluid. Here, we investigate the effects of relaxing this assumption and instead considering a friction coefficient that explicitly depends on whether the colloid is in contact with the cavity wall or not. To this end, we rewrite our governing set of equations, Eq. (6) in the main text, as

$$\begin{cases} \ddot{X} + 2B\dot{X}\left[1 - (1-\varphi)\,\delta_{\text{front contact}}\right] + \Omega_0^2\,(X - X_0)\,(\delta_{\text{front contact}} + \delta_{\text{rear contact}}) = \sin\Omega\tilde{t}, \\ \dot{V} = |\dot{X}|\,\delta_{\text{front contact}} - V. \end{cases} \tag{1}$$

Here, we have replaced the contact function used in the main text, $\delta_{\text{contact}}$, by two functions: $\delta_{\text{front contact}}$ and $\delta_{\text{rear contact}}$. The former applies if the velocity of the colloid is directed toward the cavity wall it is in contact with, whereas the latter applies if the velocity of the colloid is directed away from said wall. This distinction allows us to *only* adapt the friction coefficient if the colloid is moving into the polymer network, and not if it is moving away from it. In addition, we have recast the viscous term using a factor $1-\varphi$, which we use to compare the cases of complete screening ($\varphi = 0$), no screening ($\varphi = 1$), and reinforced friction ($\varphi = 2$). The steady-state oscillation amplitude and cavity volume corresponding to these cases are represented in Fig. 1 by the solid, dashed, and dotted curves, respectively. For this we use the same parameter values as in the main text, $\Omega_0 = 0.7$ and $B = 0.05$.

From the figure we find that the general trends of our clear scaling laws in the low- and high-frequency limits, with a pronounced resonance at intermediate frequencies (theoretical estimates not shown here), persist upon relaxing the assumption of complete screening. The decrease in resonant amplitude upon increasing $\varphi$ is expected, as this effectively makes the role of viscous friction more significant. In correspondence with out findings in the main text, this does not change the scaling laws in the low- and high-frequency limits.

In addition, we see that the finer features of the model, such as the resonance peak being split in two and the emergence of multiple local optima in the low-frequency regime, are suppressed upon increasing $\varphi$. This is likewise in line with what we reported in the main text upon varying the damping ratio $B$, and so supports the qualitative picture sketched above. That is, rendering viscous friction non-selective, or even modelling reinforced friction, does

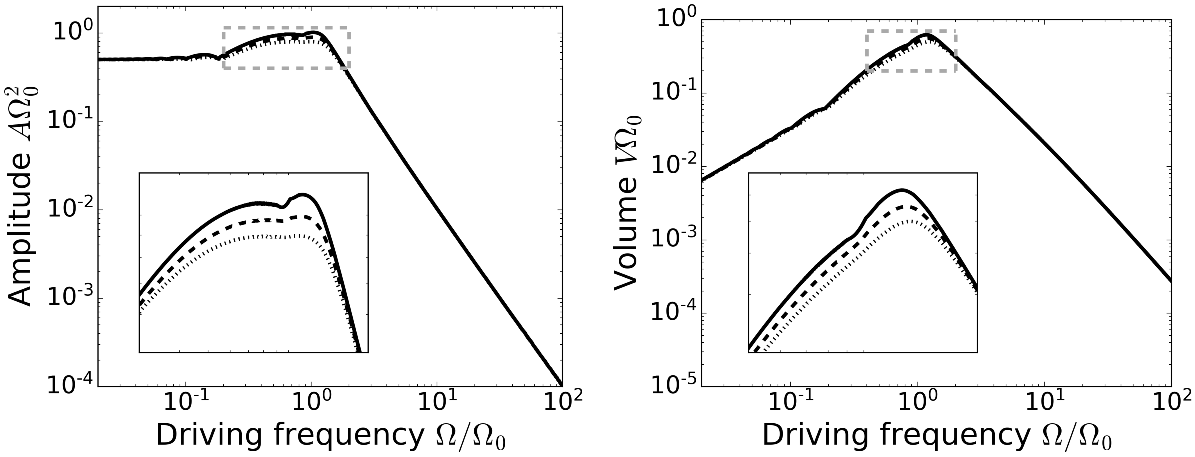


(a)

(b)

FIG. 1. Scaled steady-state amplitude, $A$, of the colloid oscillation (left) and the corresponding cavity volume, $V$, (right) as a function of the scaled driving frequency $\Omega$, on logarithmic scale. The different curves correspond to $\varphi = 0$ (solid), $\varphi = 1$ (dashed), and $\varphi = 2$ (dotted). The zoomed-in inset is indicated in grey. Parameter values used: $\Omega_0 = 0.7$ and $B = 0.05$.

not fundamentally change the model features but can be interpreted in a similar vein as tuning the system's viscosity.

## II. COLLOID DYNAMICS: FINE FEATURES

Fig. 2 presents an analogue of Fig. 2 in the main text, with the finer model features numbered one through six. For the sake of illustration, here we set $\varphi = 0$, which renders the finer model features more pronounced without fundamentally altering them.

We start by investigating the points indicated in Fig. 2(a), which shows the steady-state oscillation amplitude. The first point of interest corresponds to a driving frequency $\Omega = 3.0$, which significantly exceeds the natural frequency of the network, $\Omega_0 = 0.7$. The first panel of Fig. 3 shows the corresponding colloid oscillation, from which a competition between the driving frequency (individual oscillations) and the network's natural frequency (enveloping oscillation) is clear. The significant mismatch between the two results in an oscillation that settles to a modest amplitude in line with the high-frequency scaling relation discussed in the main text.

Following this, the second point of interest in Fig. 2(a) corresponds to a local maximum in amplitude, at $\Omega = 0.73$; the inset more clearly displays this feature. This marks the first

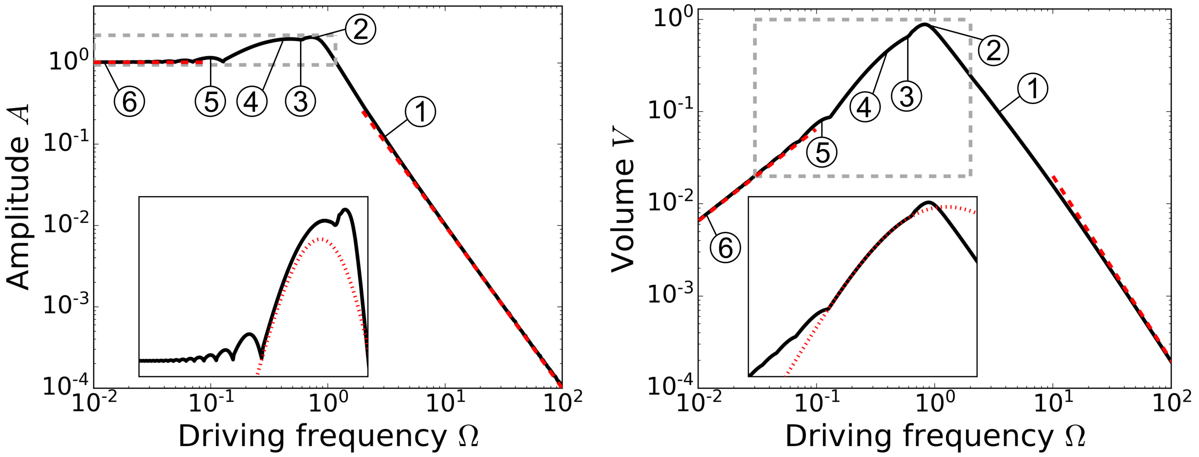


(a)

(b)

FIG. 2. Scaled steady-state amplitude, $A$, of the colloid oscillation (left) and the corresponding cavity volume, $V$, (right) as a function of the scaled driving frequency $\Omega$, on logarithmic scale. The dashed red lines denote the low- and high-frequency scaling laws explained in the main text and we use the numbers 1 through 6 to indicate points of interest in the diagram. The zoomed-in inset is indicated in grey; the dotted red curves in the insets correspond to the theoretical estimates of Eq. (7) (left) and Eq. (8) (right) in the main text, respectively. Parameter values used: $\Omega_0 = 0.5$, $B = 0.1$.

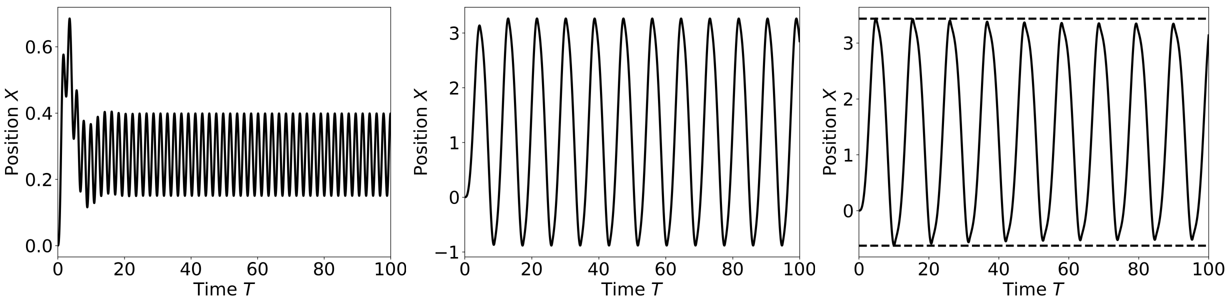


(1)

(2)

(3)

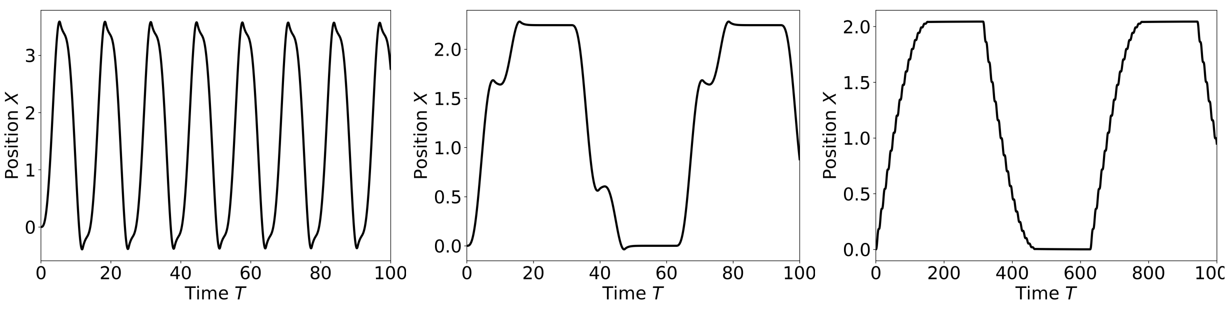


(4)

(5)

(6)

FIG. 3. Scaled colloid position $X$ as a function of the scaled time $T$. The sub-figures labelled 1 through 6 correspond to the scaled driving frequencies $\Omega = 3.0, 0.73, 0.59, 0.48, 0.10, 0.010$, respectively in Fig. 2. Parameter values used: $\Omega_0 = 0.7$, $B = 0.05$.

of multiple resonant driving frequencies, which in this case tunes into the natural frequency of the network to rapidly achieve a steady-state oscillation, as illustrated by the second panel of Fig. 3.

If we further decrease the driving frequency we find a dip in the oscillation amplitude in Fig. 2(a). The onset of this dip roughly coincides with the network's natural frequency, since for $\Omega < \Omega_0$ the turning point of the oscillation occurs before the applied field changes sign. This means that the colloid is briefly slowed down by the applied field after turning, suppressing the oscillation amplitude. This is shown by the third panel of Fig. 3, which corresponds to the dip minimum, at $\Omega = 0.59$. From the figure it is apparent that the oscillation amplitude decays as a function of time, as can be seen by comparing with the dashed black lines that show the initial amplitude. The reason the dip in the resonance curve does not extend further is because for sufficiently low driving frequencies the field repeatedly pushes the colloid back into the cavity wall, which in turn pushes back. In that case, the elastic restoring force compensates the field-induced slowing-down effect.

Upon decreasing the driving frequency further still we discover a second resonant driving frequency, $\Omega = 0.48$, which marks the fourth point of interest in Fig. 2(a). The inset shows that this resonance corresponds well with the theoretical estimate of Eq. (7) in the main text (dotted red line), suggesting the assumptions of constant contact prior to the turning point and negligible residual velocity and acceleration at the turning point are justified in this regime. It then follows that this resonance coincides with the driving frequency that maximises the position of the first turning point, as the oscillation continues identically from the point onward.

If we look at the inset of Fig. 2(a) for even lower driving frequencies, we find that an array of resonances steadily decreasing in magnitude emerges. The first of these peaks corresponds to the fifth point of interest, which no longer lies on the dotted red line of Eq. (7) in the main text. This is because for driving frequencies that are sufficiently slow compared to the network's natural frequency, the colloid undergoes multiple minor oscillations (on the network's natural time scale) before reaching its eventual turning point. The fifth panel in Fig. 3 illustrates this feature, which is not specific to our model but can be derived identically from a simple, driven harmonic oscillator.

Based on the above, it should come as no surprise that subsequent, smaller peaks in Fig. 2(a), at even lower driving frequencies, correspond to an increasing number of these

minor oscillations, $n = 1, 2, 3, ....$ The onset of these peaks follow the higher-order harmonics $\Omega = \Omega_0/(1 + 4n)$. Finally, in the low-frequency limit the trajectory of the colloid approaches a continuous curve, as shown in the sixth panel of Fig. 3, which agrees well with the low-frequency scaling relation discussed above.

This concludes the discussion of the colloid dynamics, from which we find that many of the finer model features can only be understood by considering the full dynamics, rather than solely the steady-state amplitude; this does not alter our message in the main text, however. Next, we discuss the fine features apparent from the concomitant volume expansion of the microscopic cavity.

## III. CAVITY EXPANSION: FINE FEATURES

The finer features superimposed on the steady-state cavity free volume resonance curve, as indicated by the numbered points in Fig. 2(b), follow the same trends as discussed in Sec. II. That is, for high driving frequencies (point (1)) the mismatch between driving and natural frequency leads to an erratic expansion of the microscopic cavity before it settles on its steady state, as the first panel of Fig. 4 shows. We reiterate that the frequency with which the cavity volume oscillates is twice that of the colloid oscillation, as the cavity volume is expanded upon both leftward and rightward motion.

Following this, the primary resonance in terms of volume expansion is located at the same driving frequency as the highest-frequency resonance discussed in Sec. II (point (2)). This is not surprising, as the viscoelastic relaxation of the cavity biases the results toward faster actuation. The second panel of Fig. 4 shows the corresponding expansion of the cavity volume.

Next, point (3) coincides with the dip that separates the two major resonance peaks of the model. In Sec. II, we argued that this results from to the incommensurability of the driving frequency and the network's natural frequency. The third panel of Fig. 4 shows the corresponding cavity volume, which decays in a manner similar to the colloid position in the third panel of Fig. 3.

Point (4) then marks the second resonance of the system, which is well described by the theoretical estimate of Eq. (III) (see the inset of Fig. 2(b)). The fourth panel of Fig. 4 shows the corresponding evolution of the cavity volume, which does not exhibit the distinct

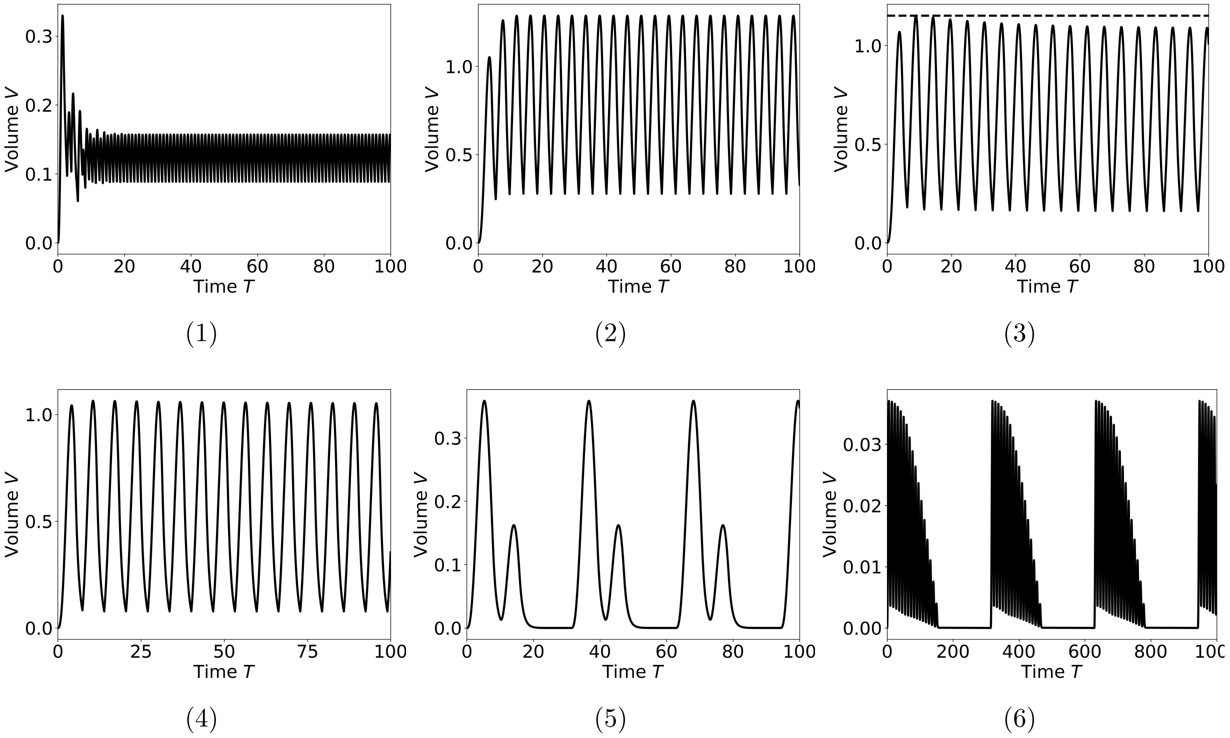


FIG. 4. Scaled cavity volume $V$ as a function of the scaled time $T$. The sub-figures labelled 1 through 6 correspond to the scaled driving frequencies $\Omega = 3.0, 0.73, 0.59, 0.48, 0.10, 0.010$, respectively (see Fig. 2(b)). Parameter values used: $\Omega_0 = 0.7$, $B = 0.05$.

decay as a function of time we discussed above.

Finally, the low-frequency limit is again characterised by the colloid undergoing multiple minor oscillations on top of the one imposed by the driving force. The fifth panel of Fig. 4 indicates that if the colloid undergoes only one such oscillation, the expansion of the cavity volume splits in two distinct stages: before and after. This is because at the point of the minor oscillation the colloid's motion is almost completely arrested, and so the cavity volume relaxes.

The sixth panel of Fig. 4 illustrates how this feature generalises to many minor oscillations, in which case the cavity volume approaches a continuous curve. The resonance peaks corresponding to these features in Fig. 2(b) are much less pronounced than for the oscillation amplitude due to the viscoelastic relaxation of the gel.

## IV. EXTERNAL FIELD: SINE VERSUS COSINE

As discussed in the main text, the fact that we allow plastic rearrangements to occur causes the eventual steady state to depend non-trivially on the transient stages of dynamics. This is because in these stages plastic rearrangements occur. Accordingly, driving the colloid with an external field in the form of a cosine yields distinct results from actuation by a sine field, since the initial "kick" provided by the former can have a large effect on which plastic rearrangements occur. Fig. 5 compares the steady states achieved by an external field in the form of a sine (grey curve) and an external field in the form of a cosine (black curve). Here we use $\varphi = 0$, as in the main text.

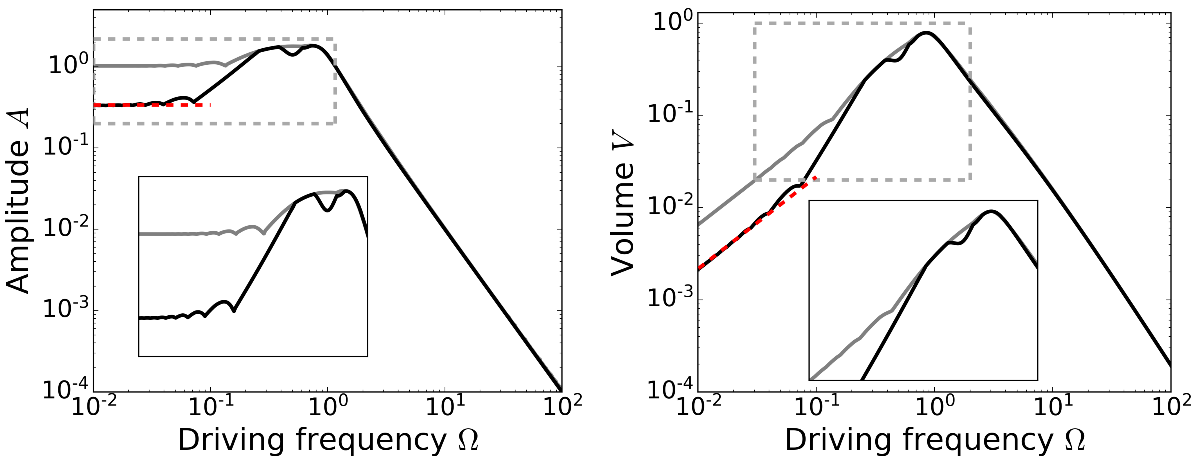


(a) (b)

FIG. 5. Scaled steady-state amplitude, $A$, of the colloid oscillation (left) and the corresponding cavity volume, $V$, (right) as a function of the scaled driving frequency $\Omega$, on logarithmic scale. The different curves correspond to an external field $\sin \Omega T$ (grey) and an external field $\cos \Omega T$ (black). The dashed red lines denote the low-frequency scaling laws discussed in the text and the zoomed-in inset is indicated in grey. Parameter values used: $\Omega_0 = 0.7$ and $B = 0.05$.

The most distinctive feature apparent from Fig. 5(a) is that the black curve (cosine actuation) lies markedly lower than the grey curve (sine actuation) in the low-frequency limit. This is because the initial "kick" provided by the cosine external field immediately induces significant plastic rearrangements. In essence, this translates the colloid to a new rest position, from which slower oscillations, like those induced by a sine external field, can subsequently take place. The key difference, however, is that this new rest position is not stress free, since elastic stresses were incurred when the colloid displaced the crosslinked

polymer gel to this new reference configuration. These stresses only relax once the external field varies sufficiently to force the colloid away from its new reference configuration. Since any ensuing oscillation must occur against the backdrop of these residual stresses, their corresponding amplitude becomes smaller.

Mathematically, turning on a cosine external field initiates a swift translation on the network's natural time scale, $1/\Omega_0$. In this case inertia cannot be neglected. Instead ignoring viscous friction, and approximating $\cos \Omega T \approx 1$, we find

$$X(T) = \frac{1}{\Omega_0^2}\left(1 - \cos \Omega_0 T\right). \tag{2}$$

The colloid follows this trajectory during its initial oscillation, freeing up a cavity of unoccupied volume in its wake. The model states that this cavity shrinks exponentially via plastic rearrangements. Subsequently, the motion of the colloid is arrested if, after passing the turning point of its oscillation, it encounters the cavity wall that is closing in due to plastic rearrangements. By using the dynamical equation for the cavity volume, we estimate this to occur at

$$X_0 = \frac{2}{\Omega_0^2} - \frac{1}{2}\frac{1 + e^{-\pi/\Omega_0}}{1 + \Omega_0^2}. \tag{3}$$

Since we assume plastic rearrangements, the colloid maintains the rest position estimated above until the external field changes direction and forces it away. In the low-frequency limit this process occurs gradually, justifying us neglecting inertia and friction henceforth. Following the line of reasoning put forth in the main text, a balance of the elastic force and and the external field then suggests that the colloid is perturbed from its rest position by $|X - X_0| = 1/\Omega_0^2$. Since the rest positions of the cavity walls are given by $X_0 = 0$ and Eq. (3), respectively, the steady-state amplitude becomes $A_{\text{low}} = \frac{1}{2}\left(1 + e^{-\pi/\Omega_0}\right)/\left(1 + \Omega_0^2\right)$, in good correspondence with Fig. 5(a) (dashed red line).

Comparing with Fig. 5(b) shows that the same discrepancy holds for the steady-state cavity free volume in the low-frequency limit. In the main text we already argued that in this regime we expect the free volume generated by colloid motion to be exactly compensated by the viscoelastic relaxation of the polymer gel in the steady state. Thus, using the estimate for the steady-state amplitude derived above we find $V_{\text{low}} = \frac{\Omega}{\pi}\left(1 + e^{-\pi/\Omega_0}\right)/\left(1 + \Omega_0^2\right)$, in good correspondence with Fig. 5(b) (dashed red line).

Fig. 5 shows that the discrepancy between the grey and the black curves shrinks as we

increase the driving frequency, and finally vanishes completely in the high-frequency limit. This is because the main feature distinguishing the two is the initial "kick" provided by the cosine external field, and the concomitant plastic rearrangements. As the oscillation of the external field is increased this effect becomes increasingly minor, becoming negligible for sufficiently high driving frequencies.

The final feature distinguishing the black curve (cosine actuation) from the grey curve (sine actuation) in both panels of Fig. 5 is that the dip splitting the resonance into two peaks is significantly more pronounced. This indicates that also the fine model features can be altered non-trivially by the plastic rearrangements that occur during the transient stages of actuation, though which features occur remains unchanged.
